# Supplementary material for: Force-Constrained Visual Policy: Safe Robot-Assisted Dressing via Multi-Modal Sensing
Source: arXiv:2311.04390 source file (2024-04-24)
Supplement: Supplementary file 1 [file appendix.tex]

\appendix

\addcontentsline{toc}{section}{Appendix} % Add the appendix text to the document TOC
\part{Appendix} % Start the appendix part

\parttoc % Insert the appendix TOC

\section{Simulation Experiment Details}
\subsection{Force Dynamics Model Training Details}
Figure~\ref{fig:force_dynamics_model} shows the architecture of the force dynamics model.
We use PointNet++~\cite{qi2017pointnet++} as the encoder for the force dynamics model. It has 2 set abstraction layers, with subsampling ratio $1, 1$ and subsampling radius $0.05, 0.01$. After the input point cloud is encoded into a latent vector, it is concatenated with the robot action and the force history. Another MLP of size $[1024, 1024]$ then takes as input the concatenated vector and outputs the force prediction of next time step.

As mentioned in the main paper, we generate 20 human meshes of varying gender, body shapes, and body sizes in simulation. For each human mesh, we collect $180$ training trajectories for $18$ different arm poses and 5 different garments as proposed in~\cite{Wang2023One}. The original paper used 27 different arm pose regions, we removed 9 of those which have upwards shoulder angles, since we find those are not practical poses for dressing through our human studies. Each training trajectory contains $150$ time steps. We train the force dynamics model with the Adam optimizer with learning rate $5 \times 10^{-4}$, and we train it with $600$ epochs to convergence. 

\subsection{Reward Function, Baselines, and Evaluation Metrics Details}
\rebuttal{\textbf{Reward function design:}
The reward function utilized in simulation to train the vision-based policy remains the same as that used in the prior work~\cite{Wang2023One}. The full reward function we use is $$r=r_m+r_p+r_c+r_d$$ We expand each term as follows:
\begin{itemize}
    \item $r_m$ measures the progression of the dressing task, which is the dressed distance along the simulated human's arm (see~\cite{Wang2023One} for more details).
    \item $r_p$ is a penalty term that helps avoiding unrealistic simulation in which the cloth penetrates through the arm when the simulation force is too large. Specifically, let $f$ be the total applied force from the garment to the human in simulation, and $f_{max}$ be the max threshold that will cause the cloth to penetrate the simulated human, this reward is computed as $r_p=-0.001 \cdot \max(f-f_{max}, 0)$. We set $f_{max}$ to be 1000 units as measured by the simulator, which is a threshold value empirically determined to be when the cloth starts penetrating into the simulated human. We note that due to simulation modeling inaccuracies, this number given by the simulator does not correspond to $1000$ Newtons of force in the real world. 
    \item The third term $r_c$ is a contact penalty term that prevents the robot end-effector from moving too close to the simulated human's arm. Let $d_e$ be the shortest distance between the end-effector and the points of the arm, this reward term is computed as $ r_c = −0.01 \cdot 1(d_e < d_{\min})$, where $1(d_e < d_{\min}) = 1$ if $d_e < d_{\min}$ and $0$ otherwise. $d_{\min}$ is set to be $1 \text{cm}$ in our experiments.
    \item The last reward term $r_d$ is a deviation penalty that discourages the sleeve from moving too far away from the simulated human's arm. Let $d_g$ be the shortest distance from the center of the shoulder part of the garment to the points of the arm, this reward is computed as $r_d = 0.02$ if $d_g < 3 \text{cm}$, $r_d = −0.05$ if $d_g > 7.5 \text{cm}$, and $r_d = 0$ otherwise.
\end{itemize}
% Note that we don't include a term that encourages force minimization when training the vision-based policy. For the \textbf{Multimodal Policy} and \textbf{Force Residual Policy} baselines, we add an additional term to the reward function to encourage lower force.
}

\textbf{Vision only baseline~\cite{Wang2023One}:} We obtain the code from the authors of~\cite{Wang2023One}. We followed all hyper-parameter settings in the original paper. 

\textbf{Force only baseline~\cite{erickson2018deep}:} Following~\cite{erickson2018deep}, actions are heuristically sampled within a forward task progression cone formed by the human's arm during data collection. The force dynamics model $d_\psi(o, F, a)$ is trained exactly the same way as our method. During test time, we plan actions according to a cost function that encourages lower force applied to the human arm and higher dressing performance. Formally, the cost function is represented by three weighted terms as follows: 
\begin{align*}
    J(o_t, F_t, a_{t}) ={}& w_1\  |d_\psi(o_t, F_t, a_t)|_1 \\ 
                                     & - w_2\ \bm{d} \cdot a_{t}^{\text{translation}} \\
                                     & + w_3\  ||a_{t}||^2_2
\end{align*}
where $\bm{d}$ is the vector from human's finger to elbow when the garment is still on forearm and from human's elbow to shoulder when the garment is on the upper arm. We use $w_1 = 0.001$, $w_2 = 1$, and $w_3 = 0.1$.

\rebuttal{\textbf{Multimodal Policy baseline:}
For this baseline, we add the force history as part of the input to the actor and critic. The force history is concatenated with the point cloud latent features that are encoded by a PoineNet++ \cite{qi2017pointnet++} encoder. We use force history length of 5. An MLP takes the concatenated feature vectors and produces the action. We train the multimodal policy to convergence in sim A using the task reward, and then transfer and finetune it in sim B. To encourage the policy to reduce force in sim B, we add a force penalty term to the reward function when finetuning the policy in sim B. The overall reward is written as $$r_t' = r_t - w\cdot \max (0, f_t-\tau)$$, where $r_t$ is the reward at time step $t$ as described in the Reward function design section, $f_t$ is the force at time step $t$, $\tau$ is the force threshold, and $w$ is the weight given to the force penalty.
}

\rebuttal{\textbf{Force Residual Policy baseline:}
For this baseline, we first train a base policy that only takes in visual observation in sim A using RL. Then in sim B, we train a separate force residual policy using RL. For the force residual policy, it takes as input the point cloud, the force history, and the base action outputted by the base vision policy. The point cloud is encoded into a latent vector using PointNet++~\cite{qi2017pointnet++}, and both the force history and the action output from the base vision policy are concatenated with the point cloud latent vector. An MLP takes the concatenated feature vector and produces the residual action. The residual action output from the force residual policy is added to the action output from the base policy as the final action. The reward for training the Force Residual Policy is the same as \textbf{Multimodal Policy}, i.e., $r_t' = r_t - w\cdot \max (0, f_t-\tau)$. 
}

\textbf{Evaluation Metrics: } We note that when computing the averaged amount of force violations and the force violation percentages, we exclude the first 25 steps of the trajectories, as during those steps the robot is still in the process of pulling the garment to reach the hand or just dressed the garment into the forearm, and there is usually very small (near to zero) force during this stage.

\begin{figure}
    \centering
    \includegraphics[width=\textwidth]{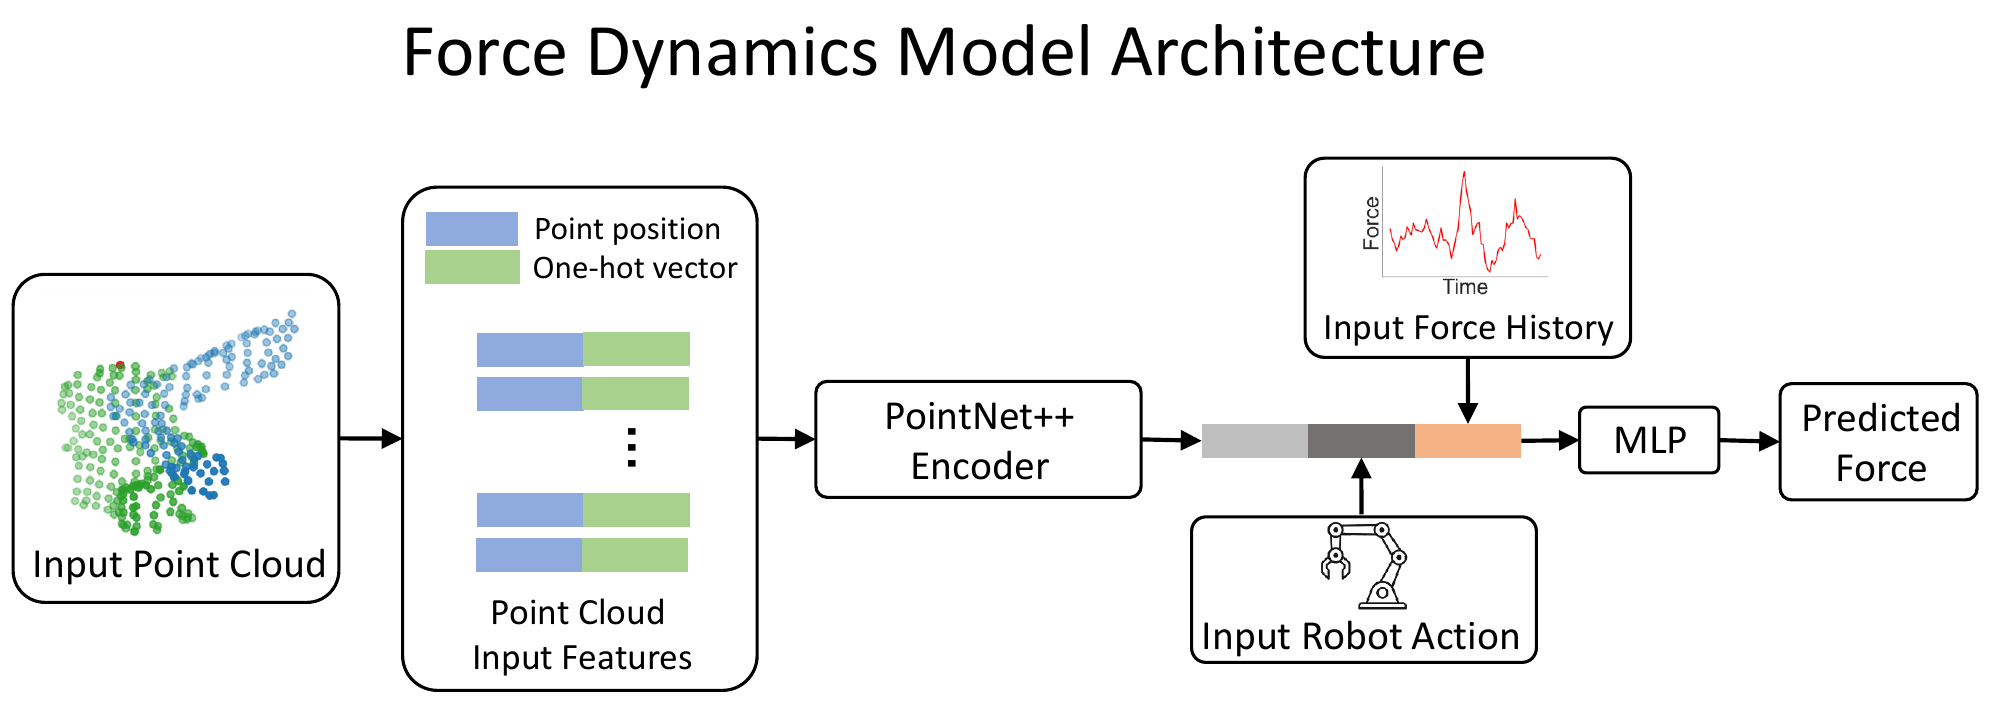}
    \caption{Force dynamics model architecture.}
    \label{fig:force_dynamics_model}
\end{figure}

% \subsection{Visuals of simulation}
% \yufei{Zhanyi: can you record a trajectory of our method and put it here?}

\section{Human Study Experiment Details}
\subsection{Trial Procedure}
We follow prior work~\cite{Wang2023One} for conducting each trials as follows. 

We first ask the participant to lift their right arm to maintain the pose they should imitate. We then record a point cloud of the participant's right arm. We then move the Sawyer's end-effector, which is already holds the garment, to be positioned near the participant's hand. We capture the point cloud of only the garment using color thresholding. 
The participant holds their arm steady throughout the trial. The static arm point cloud, the garment point cloud, and robot end-effector position, are used as input to the vision-based policy.
We run each trial to a fixed time step unless the participant wishes to have the trial stopped. After the trial terminates, we measure dressing distances to compute the whole/upper arm dressed ratio. At the end of each trial, we provide the participant with the  7-point Likert item statements. 

\subsection{Script to Participants}
Before the study, we read the following script to the participants to explain to them the study procedure:

\textit{We are conducting a study to evaluate a robot-dressing system. The robot will dress the garment on your right arm. 
We will now walk you through the steps we are taking. 
You will first read and sign the consent form, and fill in a demographic form. 
We will then measure some statistics of your arm, including the forearm length, upper arm length, and the arm circumference before the study starts.
We will put a marker on your shoulder for the experiment. 
We will then start the study. There will be a total of 24 dressing trials.
The study will be divided into two parts. The first part has 8 trials and the second part has 16 trials. After the first part is complete, we will need 10 minutes to prepare for the second part. You can take a break at that time. 
During each trial, you will be asked to hold a certain arm pose. We will test two garments and two poses during the study and we will alternate between those poses. We will show you the pose you need to hold on the screen in front of you and also demonstrate the pose by ourselves. 
You may not move once the trial starts. In each trial, we will first capture the image of your right arm, and we will move the robot closer to your hand (you may not move during the process). Then we will start the dressing, which will last 40 seconds to 1 minute. 
During dressing, the robot might pull you or tug you. In those cases, try your best not to move. If the force is too large or you feel uncomfortable, we will terminate the trial immediately. 
Occasionally there will be operation failures on us for a trial. We will repeat those trials when such failures happen. 
After each trial, please hold the arm static for another few seconds while we measure some statistics of the dressing performance. Then you can rest the arm and you will be asked to fill in three questions. The questionnaire is a likert-scale item with 3 questions. 1 is strongly disagree, 7 is strongly agree. 
You can rest whenever you feel tired, just let us know. }

\subsection{Force Model Training Details}

As mentioned in the main paper, we train personalized force dynamics model for each participant using a small amount of data (8 trials) collected on each person. The network architecture and hyper-parameters for training a force dynamics model in the real world is the same as in simulation (Figure~\ref{fig:force_dynamics_model}), except that we use a smaller learning rate of $2 \times 10^{-4}$.

%In preliminary experiments we observe that it is difficult to train a force dynamics model that can generalize to new participants given limited amount of data. We leave training a force dynamics model that generalizes across different people for future research. 
\begin{figure}[h!]
    \centering
    \includegraphics[width=0.7\textwidth]{images/real_world_res_individual_box.png}
    \vspace{0.0in}
    \caption{Box plot of the force distributions of individual participants.}
\label{fig:real_world_res_individual_box}
    \vspace{0.0in}
\end{figure}

\begin{figure}[h!]
    \centering
    \includegraphics[width=0.67\textwidth]{images/real_exp_force_traj_cmp_avg_person.png}
    \caption{Averaged forces across all 264 dressing trials in the human study.}
\label{fig:real_world_shaded_force_traj_plot}
    \vspace{0.0in}
\end{figure}

\subsection{More Results on Real-World Human Study}
Figure~\ref{fig:real_result} in the main paper shows the density plot and box plot of the force distributions on all 11 participants in the human study. We also report the force distributions on individual participants, shown by Figure~\ref{fig:real_world_res_individual_box}. For most participants, FCVP outperforms both the Vision Only and Vision w/ Random Action baseline. Figure~\ref{fig:real_world_shaded_force_traj_plot} shows the averaged force trajectory across all 264 dressing trials in the real world human study. FCVP has significantly fewer force violations compared to the baselines.
